# Supplementary material for: Measuring Domain Shifts using Deep Learning Remote Photoplethysmography Model Similarity
Source: arXiv:2404.08184 source file (2024-04-12)
Supplement: Supplementary file 1 [file appendix.tex]

\section{Appendix}

\begin{table*}
    \centering\scriptsize
    \begin{tabular}{c|ccccccc}
        \toprule
        Test Dataset     & Worst              & Average            & Best               & \texttt{DS-diff}   & \% over Worst       & \% over Average      & \% over Best         \\
        \midrule
        BP4D-1           & 8.990 $\pm$ 3.013  & 6.208 $\pm$ 0.268  & 4.917 $\pm$ 0.127  & 6.776 $\pm$ 0.754  & 0.201 $\pm$ 0.271 & -0.095 $\pm$ 0.165 & -0.379 $\pm$ 0.169 \\
        BP4D-2           & 5.717 $\pm$ 1.863  & 3.834 $\pm$ 0.101  & 2.822 $\pm$ 0.193  & 3.984 $\pm$ 0.699  & 0.262 $\pm$ 0.271 & -0.039 $\pm$ 0.179 & -0.407 $\pm$ 0.162 \\
        BP4D-3           & 4.166 $\pm$ 1.025  & 3.018 $\pm$ 0.096  & 2.338 $\pm$ 0.176  & 4.166 $\pm$ 1.025  & 0.000 $\pm$ 0.000 & -0.378 $\pm$ 0.310 & -0.795 $\pm$ 0.513 \\
        BP4D-4           & 18.481 $\pm$ 2.173 & 13.627 $\pm$ 0.383 & 11.120 $\pm$ 0.329 & 14.990 $\pm$ 2.036 & 0.186 $\pm$ 0.108 & -0.099 $\pm$ 0.129 & -0.347 $\pm$ 0.166 \\
        BP4D-5           & 6.391 $\pm$ 3.013  & 3.824 $\pm$ 0.174  & 2.474 $\pm$ 0.429  & 3.658 $\pm$ 0.363  & 0.372 $\pm$ 0.256 & 0.043 $\pm$ 0.087  & -0.490 $\pm$ 0.147 \\
        BP4D-6           & 9.556 $\pm$ 3.106  & 5.718 $\pm$ 0.230  & 4.043 $\pm$ 0.197  & 4.426 $\pm$ 0.267  & 0.513 $\pm$ 0.147 & 0.225 $\pm$ 0.056  & -0.096 $\pm$ 0.091 \\
        BP4D-7           & 8.036 $\pm$ 3.049  & 4.973 $\pm$ 0.256  & 3.288 $\pm$ 0.412  & 3.786 $\pm$ 0.200  & 0.500 $\pm$ 0.153 & 0.239 $\pm$ 0.030  & -0.160 $\pm$ 0.148 \\
        BP4D-8           & 5.625 $\pm$ 1.293  & 4.602 $\pm$ 0.106  & 3.993 $\pm$ 0.171  & 4.075 $\pm$ 0.210  & 0.257 $\pm$ 0.166 & 0.114 $\pm$ 0.062  & -0.022 $\pm$ 0.088 \\
        BP4D-9           & 7.608 $\pm$ 2.850  & 4.961 $\pm$ 0.198  & 4.094 $\pm$ 0.221  & 4.307 $\pm$ 0.184  & 0.395 $\pm$ 0.206 & 0.130 $\pm$ 0.072  & -0.054 $\pm$ 0.093 \\
        BP4D-10          & 9.168 $\pm$ 2.245  & 6.535 $\pm$ 0.166  & 5.339 $\pm$ 0.492  & 5.986 $\pm$ 0.361  & 0.327 $\pm$ 0.160 & 0.084 $\pm$ 0.046  & -0.127 $\pm$ 0.142 \\
        DDPM             & 27.419 $\pm$ 1.013 & 23.206 $\pm$ 0.291 & 18.202 $\pm$ 0.951 & 27.419 $\pm$ 1.013 & 0.000 $\pm$ 0.000 & -0.181 $\pm$ 0.034 & -0.507 $\pm$ 0.055 \\
        MSPM-adversarial & 39.252 $\pm$ 0.311 & 38.353 $\pm$ 0.054 & 36.739 $\pm$ 0.387 & 36.739 $\pm$ 0.387 & 0.064 $\pm$ 0.011 & 0.042 $\pm$ 0.010  & 0.000 $\pm$ 0.000  \\
        MSPM-game        & 8.841 $\pm$ 0.240  & 4.495 $\pm$ 0.188  & 1.850 $\pm$ 0.072  & 1.850 $\pm$ 0.072  & 0.791 $\pm$ 0.014 & 0.588 $\pm$ 0.031  & 0.000 $\pm$ 0.000  \\
        MSPM-hold        & 8.531 $\pm$ 0.540  & 5.084 $\pm$ 0.146  & 2.550 $\pm$ 0.148  & 4.234 $\pm$ 0.472  & 0.503 $\pm$ 0.058 & 0.168 $\pm$ 0.084  & -0.660 $\pm$ 0.162 \\
        MSPM-relax1      & 8.276 $\pm$ 0.485  & 4.275 $\pm$ 0.138  & 2.020 $\pm$ 0.094  & 3.243 $\pm$ 0.218  & 0.608 $\pm$ 0.034 & 0.241 $\pm$ 0.049  & -0.606 $\pm$ 0.112 \\
        MSPM-relax2      & 9.655 $\pm$ 0.558  & 5.397 $\pm$ 0.164  & 2.506 $\pm$ 0.231  & 3.560 $\pm$ 0.488  & 0.631 $\pm$ 0.050 & 0.340 $\pm$ 0.089  & -0.431 $\pm$ 0.292 \\
        MSPM-respiration & 4.801 $\pm$ 0.958  & 2.541 $\pm$ 0.121  & 1.271 $\pm$ 0.065  & 1.271 $\pm$ 0.065  & 0.729 $\pm$ 0.059 & 0.499 $\pm$ 0.045  & 0.000 $\pm$ 0.000  \\
        MSPM-videoBW     & 7.168 $\pm$ 1.233  & 4.010 $\pm$ 0.142  & 2.182 $\pm$ 0.071  & 4.136 $\pm$ 1.005  & 0.425 $\pm$ 0.081 & -0.031 $\pm$ 0.250 & -0.903 $\pm$ 0.509 \\
        MSPM-videoRGB    & 8.782 $\pm$ 0.976  & 3.540 $\pm$ 0.200  & 1.760 $\pm$ 0.088  & 2.145 $\pm$ 0.389  & 0.752 $\pm$ 0.069 & 0.391 $\pm$ 0.138  & -0.216 $\pm$ 0.176 \\
        PURE             & 6.092 $\pm$ 0.777  & 3.448 $\pm$ 0.444  & 1.960 $\pm$ 0.312  & 2.920 $\pm$ 1.136  & 0.525 $\pm$ 0.156 & 0.157 $\pm$ 0.292  & -0.534 $\pm$ 0.723 \\
        UBFC-rPPG        & 3.757 $\pm$ 1.997  & 1.951 $\pm$ 0.263  & 0.976 $\pm$ 0.282  & 0.976 $\pm$ 0.282  & 0.622 $\pm$ 0.466 & 0.484 $\pm$ 0.224  & 0.000 $\pm$ 0.000  \\
        \midrule
        Average          & 10.301 $\pm$ 1.131 & 7.314 $\pm$ 0.136  & 5.545 $\pm$ 0.096  & 6.888 $\pm$ 0.182  & 0.412 $\pm$ 0.083 & 0.139 $\pm$ 0.028  & -0.321 $\pm$ 0.049 \\
        \bottomrule
    \end{tabular}
    \caption{Performance of \texttt{DS-diff} for model selection.}
    \label{tab:app:ds-diff}
\end{table*}
